# Supplementary material for: Leveraging Vision-Language Models for Improving Domain Generalization in Image Classification
Source: arXiv:2310.08255 source file (2024-03-09)
Supplement: Supplementary file 1 [file distill_ext_comp.tex]

\begin{table}[t]
\centering
\caption{\textbf{Distillation to lower capacity student models (extended comparisons):} Performance (\%) of the proposed approach VL2V-ADiP (denoted as
Ours), when compared to the KD and ERM finetune baselines with SWAD (S), with different student architectures. The teacher architecture is ViT-B/16 in all cases.}
\label{tab:distill_ext_comp}
\resizebox{\linewidth}{!}{%
\begin{tabular}{@{}cccccccc@{}}

\toprule
\textbf{Student} & \textbf{Method} & \textbf{OH} & \textbf{TI} & \textbf{VLCS} & \textbf{PACS} & \textbf{DN} & \textbf{Avg. (OOD)} \\ \midrule

\multirow{3}{*}{\begin{tabular}[c]{@{}c@{}}ViT-B/16\\ (86M)\end{tabular}} & ERM (S) & 83.22 & 50.05 & 80.33 & 90.28 & 56.10 & 72.00 \\
 & KD (S) & 82.73 & 48.40 & 80.48 & 91.46 & 56.17 & 71.85 \\
 & Ours & \textbf{85.74} & \textbf{55.43} & \textbf{81.90} & \textbf{94.94} & \textbf{59.38} & \textbf{75.48} \\ \midrule

\multirow{3}{*}{\begin{tabular}[c]{@{}c@{}}ViT-S/16\\ (22M)\end{tabular}} & ERM (S) & 78.58 & 49.40 & 78.72 & 85.80 & 52.09 & 68.92 \\
 & KD (S) & 78.14 & 50.11 & 79.14 & 85.97 & 52.05 & 69.08 \\
 & Ours & \textbf{81.22} & \textbf{52.47} & \textbf{81.44} & \textbf{89.32} & \textbf{54.23} & \textbf{71.73} \\ \midrule

\multirow{3}{*}{\begin{tabular}[c]{@{}c@{}}DeiT-S/16\\ (22M)\end{tabular}} & ERM (S) & 74.95 & 47.85 & 79.37 & \textbf{89.22} & 49.18 & 68.12 \\
 & KD (S) & 74.65 & 48.11 & 78.86 & 88.14 & 49.10 & 67.77 \\
 & Ours & \textbf{77.63} & \textbf{48.72} & \textbf{81.89} & 88.97 & \textbf{50.37} & \textbf{69.52} \\ \midrule

\multirow{3}{*}{\begin{tabular}[c]{@{}c@{}}ResNet-50\\ (26M)\end{tabular}} & ERM (S) & 70.85 & 49.47 & \textbf{79.50} & \textbf{88.05} & 46.43 & 66.86 \\
 & KD (S) & 70.67 & 51.22 & 78.63 & 87.23 & 46.31 & 66.81 \\
 & Ours & \textbf{74.42} & \textbf{53.46} & 79.23 & 86.72 & \textbf{47.74} & \textbf{68.31} \\ \bottomrule
\end{tabular}%
}
\end{table}
