# Supplementary material for: Leveraging Vision-Language Models for Improving Domain Generalization in Image Classification
Source: arXiv:2310.08255 source file (2024-03-09)
Supplement: Supplementary file 2 [file dom_split_dn_ad.tex]

\label{tab:ad_dom_split}
\resizebox{\textwidth}{!}{%
\begin{tabular}{@{}lcccccccc@{}}

\toprule
\multicolumn{1}{c}{\textbf{Method}} & \textbf{Clipart} & \textbf{Infograph} & \textbf{Painting} & \textbf{Quickdraw} & \textbf{Real} & \textbf{Sketch} & \textbf{Avg.} \\ \midrule
ERM-LP & & & & & & &\\
ERM Full Fine-Tuning & 76.34 & 30.92 & 64.76 & 21.30 & 77.70 & 65.60 & 56.10 \\
LP-FT \cite{LP-FT} & & & & & & & \\
SimKD \cite{SimKD} & & & & & & & \\
KD \cite{hinton2015distilling} & 76.56 & 31.29 & 64.55 & \textbf{21.44} & 77.62 & 65.23 & 56.11 \\
MIRO \cite{MIRO} & 76.32 & 30.96 & 64.52 & 20.18 & 77.88 & 64.63 & 55.75 \\
DART \cite{DART} & 77.62	& 34.14	& 67.64	& 21.05	& 80.73	& 67.11	& 58.05 \\
SAGM \cite{SAGM} & 76.67	& 29.85	& 64.42	& 20.68	& 77.58	& 64.58	& 55.63 \\
Text2Concept \cite{SAGM} & & & & & & & \\
RISE \cite{RISE} & & & & & & & \\
\textbf{VL2V-ADiP (Ours)} & \textbf{78.80} & \textbf{36.86} & \textbf{69.21} & 21.32 & \textbf{81.33} & \textbf{68.79} & \textbf{59.38} \\ \bottomrule
\end{tabular}%
}
