# Supplementary material for: Leveraging Vision-Language Models for Improving Domain Generalization in Image Classification
Source: arXiv:2310.08255 source file (2024-03-09)
Supplement: Supplementary file 3 [file dom_split_dn_sd.tex]

\label{tab:sd_dom_split}
\resizebox{\textwidth}{!}{%
\begin{tabular}{@{}lccccccc@{}}

\toprule
\multicolumn{1}{c}{\textbf{Method}} & \textbf{Clipart} & \textbf{Infograph} & \textbf{Painting} & \textbf{Quickdraw} & \textbf{Real} & \textbf{Sketch} & \textbf{Avg.} \\ \midrule

Zero-Shot \cite{CLIP} & 72.61 & 47.08 & 66.02 & 14.13 & \textbf{83.12} & 63.18 & 57.69 \\
ERM Full Fine-Tuning & 77.10 & 38.32 & 66.13 & \textbf{25.02} & 75.19 & 65.76 & 57.92 \\
MIRO \cite{MIRO} & 79.70 & 43.50 & 67.36 & 24.62 & 79.22 & 68.42 & 60.47 \\
DART \cite{DART} & 78.51	& 39.99	& 66.89	& 25.85	& 76.37	& 68.29	& 59.32 \\
SAGM \cite{SAGM} & 78.78	& 40.21	& 67.31	& 24.18	& 76.29	& 67.54	& 59.05 \\
LP-FT \cite{LP-FT} & & & & & \\
FLYP \cite{FLYP} & & & & & \\
CLIPood \cite{CLIPood} & & & & & \\
WiSE-FT \cite{WISE-FT} & & & & & \\
RISE \cite{RISE} & & & & & \\
\textbf{VL2V-SD (Ours)} & \textbf{79.96} & \textbf{49.00} & \textbf{71.05} & 23.34 & 82.05 & \textbf{71.36} & \textbf{62.79} \\ \bottomrule

\end{tabular}%
}
