# Supplementary material for: Leveraging Vision-Language Models for Improving Domain Generalization in Image Classification
Source: arXiv:2310.08255 source file (2024-03-09)
Supplement: Supplementary file 4 [file dom_split_pacs_ad.tex]

\resizebox{\linewidth}{!}{%
\begin{tabular}{lccccc}
\toprule
\multicolumn{1}{c}{\textbf{Method}} & \textbf{Art} & \textbf{Cartoon} & \textbf{Photo} & \textbf{Sketch} & \textbf{Avg.} \\ \midrule

ERM-LP & & & & & \\
ERM Full Fine-Tuning & 93.78 & 86.25 & 99.18 & 81.93 & 90.28 \\
LP-FT \cite{LP-FT} & & & & & \\
SimKD \cite{SimKD} & & & & & \\
KD \cite{hinton2015distilling} & 94.20 & 86.35 & 99.25 & 86.04 & 91.46 \\
MIRO \cite{MIRO} & 94.69 & 85.98 & 99.63 & 77.70 & 89.50 \\
DART \cite{DART} & 94.45	& 86.67	& 99.55	& 81.52	& 90.55 \\
SAGM \cite{SAGM} & 93.72	& 86.57	& 99.18	& 80.63	& 90.02 \\
Text2Concept \cite{text2concept} & & & & & \\
RISE \cite{RISE} & & & & & \\
\textbf{VL2V-ADiP (Ours)} & \textbf{95.61} & \textbf{92.38} & \textbf{99.85} & \textbf{88.68} & \textbf{94.13} \\ \bottomrule
\end{tabular}%
}
