# Supplementary material for: Leveraging Vision-Language Models for Improving Domain Generalization in Image Classification
Source: arXiv:2310.08255 source file (2024-03-09)
Supplement: Supplementary file 5 [file dom_split_pacs_sd.tex]

\resizebox{\linewidth}{!}{%
\begin{tabular}{lccccc}

\toprule
\multicolumn{1}{c}{\textbf{Method}} & \textbf{Art} & \textbf{Cartoon} & \textbf{Photo} & \textbf{Sketch} & \textbf{Avg.} \\ \midrule

Zero-Shot \cite{CLIP} & 97.44 & \textbf{99.31} & \textbf{99.93} & 89.44 & 96.53 \\
ERM Full Fine-Tuning & 91.34 & 89.07 & 97.53 & 87.47 & 91.35 \\
MIRO \cite{MIRO} & \textbf{98.05} & 97.50 & 99.78 & 90.46 & 96.44 \\
DART \cite{DART} & 94.45 & 92.27 & 98.80 & 88.20 & 93.43 \\
SAGM \cite{SAGM} & 95.18	& 93.60	& 99.03	& 89.41	& 94.30 \\
LP-FT \cite{LP-FT} & & & & & \\
FLYP \cite{FLYP} & & & & & \\
CLIPood \cite{CLIPood} & & & & & \\
WiSE-FT \cite{WISE-FT} & & & & & \\
RISE \cite{RISE} & & & & & \\
\textbf{VL2V-SD (Ours)} & \textbf{98.05} & 98.19 & \textbf{99.93} & \textbf{90.55} & \textbf{96.68} \\
\bottomrule
\end{tabular}%
}
