# Supplementary material for: Leveraging Vision-Language Models for Improving Domain Generalization in Image Classification
Source: arXiv:2310.08255 source file (2024-03-09)
Supplement: Supplementary file 6 [file dom_split_ti_ad.tex]

\resizebox{\linewidth}{!}{%
\begin{tabular}{lccccc}
\toprule
\multicolumn{1}{c}{\textbf{Method}} & \textbf{L100} & \textbf{L38} & \textbf{L43} & \textbf{L46} & \textbf{Avg.} \\ \midrule

ERM-LP & & & & & \\
ERM Full Fine-Tuning & 58.98 & 37.76 & 58.31 & 45.15 & 50.05 \\
LP-FT \cite{LP-FT} & & & & & \\
SimKD \cite{SimKD} & & & & & \\
KD \cite{hinton2015distilling} & 61.09 & 33.21 & 57.84 & 41.17 & 48.33 \\
MIRO \cite{MIRO} & 61.27 & 38.14 & 57.68 & 44.08 & 50.30 \\
DART \cite{DART} & 56.82	& 37.34	& \textbf{62.31} & 42.26 & 49.68 \\
SAGM \cite{SAGM} & \textbf{64.17} & 44.42 & 59.64 & 44.74 & 53.24 \\
Text2Concept \cite{text2concept} & & & & & \\
RISE \cite{RISE} & & & & & \\
\textbf{VL2V-ADiP (Ours)} & 62.93 & \textbf{44.83} & 60.71 & \textbf{53.26} & \textbf{55.43} \\
\bottomrule
\end{tabular}%
}
