# Supplementary material for: Leveraging Vision-Language Models for Improving Domain Generalization in Image Classification
Source: arXiv:2310.08255 source file (2024-03-09)
Supplement: Supplementary file 7 [file dom_split_ti_sd.tex]

\resizebox{\linewidth}{!}{%
\begin{tabular}{lccccc}
\toprule
\multicolumn{1}{c}{\textbf{Method}} & \textbf{L100} & \textbf{L38} & \textbf{L43} & \textbf{L46} & \textbf{Avg.} \\ \midrule

Zero-Shot \cite{CLIP} & 51.65 & 20.03 & 33.60 & 31.49 & 34.19 \\
ERM Full Fine-Tuning & 38.94 & 38.03 & 54.03 & 40.68 & 42.92 \\
MIRO \cite{MIRO} & 67.15 & \textbf{50.75} & \textbf{66.63} & 52.71 & \textbf{59.31} \\
DART \cite{DART} & 56.82	& 37.34	& 62.31	& 42.26	& 49.68 \\
SAGM \cite{SAGM} & 72.21	& 50.10	& 62.50	& 49.73	& 58.64 \\
LP-FT \cite{LP-FT} & & & & & \\
FLYP \cite{FLYP} & & & & & \\
CLIPood \cite{CLIPood} & & & & & \\
WiSE-FT \cite{WISE-FT} & & & & & \\
RISE \cite{RISE} & & & & & \\
\textbf{VL2V-SD (Ours)} & \textbf{69.10} & 48.40 & 63.10 & \textbf{53.56} & 58.54 \\
\bottomrule
\end{tabular}%
}
