# Supplementary material for: Leveraging Vision-Language Models for Improving Domain Generalization in Image Classification
Source: arXiv:2310.08255 source file (2024-03-09)
Supplement: Supplementary file 8 [file dom_split_vlcs_ad.tex]

\resizebox{\linewidth}{!}{%
\begin{tabular}{lccccc}

\toprule
\multicolumn{1}{c}{\textbf{Method}} & \textbf{Caltech} & \textbf{LabelMe} & \textbf{VOC07} & \textbf{SUN09} & \textbf{Avg.} \\ \midrule

ERM-LP & & & & & \\
ERM Full Fine-Tuning & 98.49 & 64.05 & 82.60 & 76.17 & 80.33 \\
LP-FT \cite{LP-FT} & & & & & \\
SimKD \cite{SimKD} & & & & & \\
KD \cite{hinton2015distilling} & 98.87 & 65.32 & 81.33 & 76.39 & 80.48 \\
MIRO \cite{MIRO} & \textbf{99.75} & 64.79 & 82.66 & 77.20 & 81.10 \\
DART \cite{DART} & 94.08	& 63.11	& 76.12	& 75.86	& 77.29 \\
SAGM \cite{SAGM} & 98.49	& 64.92	& 79.32	& 75.68	& 79.60 \\
Text2Concept \cite{text2concept} & & & & & \\
RISE \cite{RISE} & & & & & \\
\textbf{VL2V-ADiP (Ours)} & 99.62 & \textbf{66.60} & \textbf{82.87} & \textbf{78.46} & \textbf{81.89} \\ \bottomrule
\end{tabular}%
}
