# Supplementary material for: Leveraging Vision-Language Models for Improving Domain Generalization in Image Classification
Source: arXiv:2310.08255 source file (2024-03-09)
Supplement: Supplementary file 9 [file dom_split_vlcs_sd.tex]

\resizebox{\linewidth}{!}{%
\begin{tabular}{lccccc}

\toprule
\multicolumn{1}{c}{\textbf{Method}} & \textbf{Caltech} & \textbf{LabelMe} & \textbf{VOC07} & \textbf{SUN09} & \textbf{Avg.} \\ \midrule

Zero-Shot & \textbf{100.00} & \textbf{69.02} & 84.19 & 74.86 & 82.02 \\
ERM Full Fine-Tuning & 99.12 & 63.31 & 79.01 & 75.08 & 79.13 \\
MIRO \cite{MIRO} & 97.53 & 66.59 & 81.57 & \textbf{83.53} & 82.30 \\
DART \cite{SWAD} & 99.12 & 65.73 & 81.07 & 75.63 & 80.38 \\
SAGM \cite{SAGM} & 97.73 & 65.86 & 83.77 & 80.85 & 82.05 \\
LP-FT \cite{LP-FT} & & & & & \\
FLYP \cite{FLYP} & & & & & \\
CLIPood \cite{CLIPood} & & & & & \\
WiSE-FT \cite{WISE-FT} & & & & & \\
RISE \cite{RISE} & & & & & \\
\textbf{VL2V-SD (Ours)} & 99.24 & 67.81 & \textbf{86.89} & 79.05 & \textbf{83.25} \\
\bottomrule
\end{tabular}%
}
